# Supplementary material for: Integrated photonic nonreciprocal devices based on susceptibility-programmable medium
Source: arXiv:2409.01106 source file (2024-09-02)
Supplement: Supplementary file 1 [file Supplementary_Materials.pdf]

# Supplementary Materials: Integrated photonic nonreciprocal devices based on susceptibility-programmable medium


Yan-Lei Zhang,[1,2,*] Ming Li,[1,2,*] Xin-Biao Xu,[1,2] Zhu-Bo Wang,[1,2] Chun-Hua Dong,[1,2,3] Guang-Can Guo,[1,2] Chang-Ling Zou,[1,2,3,†] and Xu-Bo Zou[1,2,3,‡]

[1]*CAS Key Laboratory of Quantum Information, University of Science and Technology of China, Hefei, Anhui 230026, China*
[2]*CAS Center For Excellence in Quantum Information and Quantum Physics, University of Science and Technology of China, Hefei, Anhui 230026, China*
[3]*Hefei National Laboratory, University of Science and Technology of China, Hefei 230088, China.*


## I. THEORETICAL MODEL

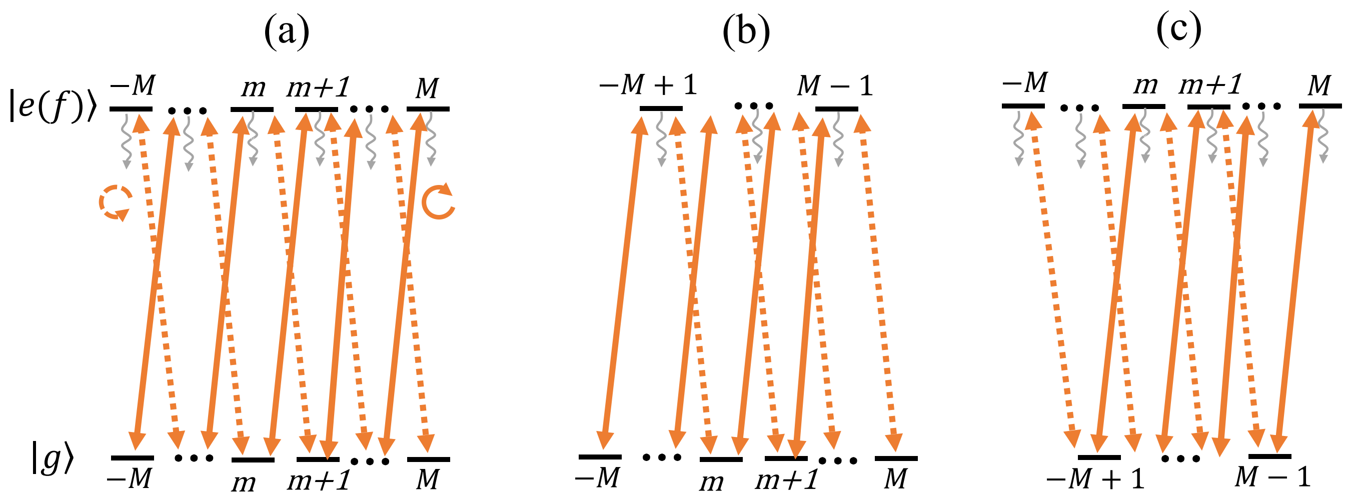


FIG. S1. Schematic of the general energy levels following the transition selection rule of $m \leftrightarrows m+1$ for the chiral field $\circlearrowright$ ($\circlearrowleft$), where $-M,...,m,m+1,...,M$ are Zeeman levels. Our model can work the general energy level stracture: (a) the Zeeman levels of the ground sate are equal to that of the excited states; (b) the Zeeman levels of the ground sate are more than that of the excited states; (c) the Zeeman levels of the ground sate are less than that of the excited states.

For a general three-level structure with energy levels $|e\rangle$, $|f\rangle$, and $|g\rangle$, the control light $\Omega$ and the signal light $E$ are used to realize the atomic transitions $|e\rangle \leftrightarrows |g\rangle$ and $|f\rangle \leftrightarrows |g\rangle$, respectively, as shown in Fig. S1. Our model is not limited to that the Zeeman levels of the ground sate are equal to that of the excited states in Fig. S1(a), and can also work for the general energy level stracture, where the Zeeman levels of the ground sate are more or less than that of the excited states in Fig. S1(b) and (c).

In the following, we take the simplified model by treating the atom as two degenerate fine levels $\pm M$, and thus the chiral light can be decomposed into right-polarized light $\circlearrowright$ and left-polarized light $\circlearrowleft$. This model can be can be described by the following Hamiltonian ($\hbar = 1$) [1]

$$\begin{aligned} H &= \sum_{j=g,f,e} \omega_j \left(\sigma_{jj}^{-M,-M} + \sigma_{jj}^{M,M}\right) + \left(\Omega_{\circlearrowleft}\sigma_{ge}^{-M,M} + \Omega_{\circlearrowright}\sigma_{ge}^{M,-M}\right) e^{i\omega_\Omega t} + \text{H.c.} \\ &\quad + \left(E_{\circlearrowright}\sigma_{gf}^{-M,M} + E_{\circlearrowleft}\sigma_{gf}^{M,-M}\right) e^{i\omega_s t} + \text{H.c.}, \end{aligned} \tag{S.1}$$

where $\sigma_{jj'}^{\pm M,\mp M} = |j,\pm M\rangle\langle j',\mp M|$ with $j, j' \in \{g, f, e\}$, and $\omega_\Omega$ and $\omega_s$ are frequencies of the control field and signal field, respectively. In the interaction picture $H_0 = \omega_\Omega \left(\sigma_{ee}^{-M,-M} + \sigma_{ee}^{M,M}\right) + \omega_s \left(\sigma_{ee}^{-M,-M} + \sigma_{ee}^{M,M}\right)$, we can obtain the interaction Hamiltonian:

$$
\begin{aligned}
H_{\mathrm{int}} \;=\; & \omega_g \left(\sigma_{gg}^{-M,-M} + \sigma_{gg}^{M,M}\right) + \left(\omega_e - \omega_\Omega\right)\left(\sigma_{ee}^{-M,-M} + \sigma_{ee}^{M,M}\right) + \left(\omega_f - \omega_s\right)\left(\sigma_{ff}^{-M,-M} + \sigma_{ff}^{M,M}\right) \\
& + \left(\Omega_{\circlearrowright}\sigma_{ge}^{-M,M} + \Omega_{\circlearrowleft}\sigma_{ge}^{M,-M}\right) + \left(E_{\circlearrowright}\sigma_{gf}^{-M,M} + E_{\circlearrowleft}\sigma_{gf}^{M,-M}\right) + \mathrm{H.c.}, \qquad \text{(S.2)}
\end{aligned}
$$

and the corresponding master equation can be written as

$$
\frac{d\rho}{dt} = -i[H,\rho] + \gamma_{ge}^{mn}\mathscr{L}\left(\sigma_{ge}^{\pm M \mp M}\right) + \gamma_{gf}^{\pm M \mp M}\mathscr{L}\left(\sigma_{gf}^{\pm M \mp M}\right), \qquad \text{(S.3)}
$$

where $\gamma_{ge(f)}^{\pm M \mp M}$ is the decay rate and the Lindblad super-operatior $\mathscr{L}(o) = o\rho o^{\dagger} - \rho o^{\dagger} o/2 - o^{\dagger} o\rho/2$. For simplification, we assume $\gamma_{ge(f)}^{\pm M \mp M} = \gamma$. In our scheme, we have $\Omega \gg E$, which means that the atomic populations are mainly determined by the control field. According to the master equation, the dynamics of the system can be described by the following equations:

$$
\begin{aligned}
\frac{d}{dt}\sigma_{\mathrm{ee}}^{M,M} &= -i\Omega_{\circlearrowright}\left(\sigma_{\mathrm{eg}}^{M,-M} - \sigma_{\mathrm{ge}}^{-M,M}\right) - 2\gamma\sigma_{\mathrm{ee}}^{MM}, & \text{(S.4)} \\
\frac{d}{dt}\sigma_{\mathrm{ee}}^{-M,-M} &= -i\Omega_{\circlearrowleft}\left(\sigma_{\mathrm{eg}}^{-M,M} - \sigma_{\mathrm{ge}}^{M,-M}\right) - 2\gamma\sigma_{\mathrm{ee}}^{-M,-M}, & \text{(S.5)} \\
\frac{d}{dt}\sigma_{\mathrm{gg}}^{-M,-M} &= -i\Omega_{\circlearrowright}\left(\sigma_{\mathrm{ge}}^{-M,M} - \sigma_{\mathrm{eg}}^{M,-M}\right) + \gamma\left(\sigma_{\mathrm{ee}}^{M,M} + \sigma_{\mathrm{ee}}^{-M,-M}\right), & \text{(S.6)} \\
\frac{d}{dt}\sigma_{\mathrm{gg}}^{M,M} &= -i\Omega_{\circlearrowleft}\left(\sigma_{\mathrm{ge}}^{M,-M} - \sigma_{\mathrm{eg}}^{-M,M}\right) + \gamma\left(\sigma_{\mathrm{ee}}^{M,M} + \sigma_{\mathrm{ee}}^{-M,-M}\right), & \text{(S.7)} \\
\frac{d}{dt}\sigma_{\mathrm{eg}}^{M,-M} &= -i\Delta\sigma_{\mathrm{eg}}^{M,-M} - i\Omega_{\circlearrowright}\left(\sigma_{\mathrm{ee}}^{M,M} - \sigma_{\mathrm{gg}}^{-M,-M}\right) - \gamma\sigma_{\mathrm{eg}}^{M,-M}, & \text{(S.8)} \\
\frac{d}{dt}\sigma_{\mathrm{eg}}^{-M,M} &= -i\Delta\sigma_{\mathrm{eg}}^{-M,M} - i\Omega_{\circlearrowleft}\left(\sigma_{\mathrm{ee}}^{-M,-M} - \sigma_{\mathrm{gg}}^{M,M}\right) - \gamma\sigma_{\mathrm{eg}}^{-M,M}. & \text{(S.9)}
\end{aligned}
$$

Here, $\Delta = \omega_g - \omega_f + \omega_\Omega$ is the laser detuning with respect to the transition. In the steady states, we can obtain the populations are

$$
\begin{aligned}
\sigma_{gg}^{-M,-M} &= \frac{\left(\gamma^2 + \Delta^2 + \Omega_{\circlearrowright}^2\right)\Omega_{\circlearrowleft}^2}{\left(\gamma^2 + \Delta^2\right)\left(\Omega_{\circlearrowright}^2 + \Omega_{\circlearrowleft}^2\right) + 4\Omega_{\circlearrowright}^2\Omega_{\circlearrowleft}^2}, & \text{(S.10)} \\
\sigma_{gg}^{M,M} &= \frac{\left(\gamma^2 + \Delta^2 + \Omega_{\circlearrowleft}^2\right)\Omega_{\circlearrowright}^2}{\left(\gamma^2 + \Delta^2\right)\left(\Omega_{\circlearrowright}^2 + \Omega_{\circlearrowleft}^2\right) + 4\Omega_{\circlearrowright}^2\Omega_{\circlearrowleft}^2}. & \text{(S.11)}
\end{aligned}
$$

Here we consider the susceptivity of the signal field $E$, we can obtain the dynamical equations

$$
\begin{aligned}
\frac{d\sigma_{fg}^{M,-M}}{dt} &= -i\delta\sigma_{fg}^{M,-M} - i\Omega_{\circlearrowright}\sigma_{fe}^{M,M} - iE_{\circlearrowright}\left(\sigma_{ff}^{M,M} - \sigma_{gg}^{-M,-M}\right) - \gamma\sigma_{fg}^{M,-M}, & \text{(S.12)} \\
\frac{d\sigma_{fg}^{-M,M}}{dt} &= -i\delta\sigma_{fg}^{-M,M} - i\Omega_{\circlearrowleft}\sigma_{fe}^{-M,-M} - iE_{\circlearrowleft}\left(\sigma_{ff}^{-M,-M} - \sigma_{gg}^{M,M}\right) - \gamma\sigma_{fg}^{-M,M}, & \text{(S.13)}
\end{aligned}
$$

where $\delta = \omega_g - \omega_f + \omega_s$.If $\gamma > \Omega \gg E$, we can ignore the transition $|e\rangle \leftrightarrows |f\rangle$. The steady-state solutions can be written as

$$
\begin{aligned}
\sigma_{fg}^{M,-M} &\approx \frac{iE_{\circlearrowright}\left(-\sigma_{ff}^{M,M} + \sigma_{gg}^{-M,-M}\right)}{i\delta + \gamma}, & \text{(S.14)} \\
&\approx \frac{iE_{\circlearrowright}}{i\delta + \gamma}\frac{\left(\gamma^2 + \Delta^2 + \Omega_{\circlearrowright}^2\right)\Omega_{\circlearrowleft}^2}{\left(\gamma^2 + \Delta^2\right)\left(\Omega_{\circlearrowright}^2 + \Omega_{\circlearrowleft}^2\right) + 4\Omega_{\circlearrowright}^2\Omega_{\circlearrowleft}^2} & \text{(S.15)} \\
\sigma_{fg}^{-M,M} &\approx \frac{iE_{\circlearrowleft}\left(-\sigma_{ff}^{-M,-M} + \sigma_{gg}^{M,M}\right)}{i\delta + \gamma}, & \text{(S.16)} \\
&\approx \frac{iE_{\circlearrowleft}}{i\delta + \gamma}\frac{\left(\gamma^2 + \Delta^2 + \Omega_{\circlearrowleft}^2\right)\Omega_{\circlearrowright}^2}{\left(\gamma^2 + \Delta^2\right)\left(\Omega_{\circlearrowright}^2 + \Omega_{\circlearrowleft}^2\right) + 4\Omega_{\circlearrowright}^2\Omega_{\circlearrowleft}^2}. & \text{(S.17)}
\end{aligned}
$$

Here we assumed that $\sigma_{ff}^{-(+)M,-(+)M} \ll \sigma_{gg}^{-(+)M,-(+)M}$, and the approximate analytical solutions can be obtained. The corresponding susceptibility [1, 2] is defined as

$$\chi_{\circlearrowright(\circlearrowleft)} = \frac{\rho \left|\mu_{fg}\right|^2 \sigma_{fg}^{+(-)M,-(+)M}}{\varepsilon_0 \hbar E_{\circlearrowright(\circlearrowleft)}}, \tag{S.18}$$

that is,

$$\chi_{\circlearrowright} \approx \frac{i\rho \left|\mu_{fg}\right|^2}{(i\delta+\gamma)\,\varepsilon_0\hbar} \frac{\left(\gamma^2+\Delta^2+\Omega_{\circlearrowright}^2\right)\Omega_{\circlearrowleft}^2}{\left(\gamma^2+\Delta^2\right)\left(\Omega_{\circlearrowright}^2+\Omega_{\circlearrowleft}^2\right)+4\Omega_{\circlearrowright}^2\Omega_{\circlearrowleft}^2}, \tag{S.19}$$

$$\chi_{\circlearrowleft} \approx \frac{i\rho \left|\mu_{fg}\right|^2}{(i\delta+\gamma)\,\varepsilon_0\hbar} \frac{\left(\gamma^2+\Delta^2+\Omega_{\circlearrowleft}^2\right)\Omega_{\circlearrowright}^2}{\left(\gamma^2+\Delta^2\right)\left(\Omega_{\circlearrowright}^2+\Omega_{\circlearrowleft}^2\right)+4\Omega_{\circlearrowright}^2\Omega_{\circlearrowleft}^2}, \tag{S.20}$$

where $\rho$ is the atomic density. It is obvious that the susceptibility of the weak signal field is fully determined by the control field $\Omega_{\circlearrowright}$ and $\Omega_{\circlearrowleft}$. When $\Omega_{\circlearrowright} \neq \Omega_{\circlearrowleft}$, the dispersion or absorption is different for different circularly polarized fields, where $\chi_{\circlearrowright} \neq \chi_{\circlearrowleft}$. The difference is actually related to the nonreciprocity for the transmitting light.

To show the nonreciprocal property better, we consider a weak signal field $E$ travelling along the $z$ axis, and we note that $E_{\circlearrowright(\circlearrowleft)} = \left[E_x + (-)\, iE_y\right]/\sqrt{2}$. Therefore the representation of the polarization can be transformed to Cartesian coordinates as follows

$$\begin{aligned}
\begin{pmatrix} P_x \\ P_y \end{pmatrix} &= \frac{\varepsilon_0}{2} \begin{pmatrix} 1 & 1 \\ -i & i \end{pmatrix} \begin{pmatrix} \chi_{\circlearrowright} & 0 \\ 0 & \chi_{\circlearrowleft} \end{pmatrix} \begin{pmatrix} 1 & i \\ 1 & -i \end{pmatrix} \begin{pmatrix} E_x \\ E_y \end{pmatrix} \\
&= \frac{\varepsilon_0}{2} \begin{pmatrix} \chi_{\circlearrowright} + \chi_{\circlearrowleft} & -i\left(\chi_{\circlearrowleft} - \chi_{\circlearrowright}\right) \\ i\left(\chi_{\circlearrowleft} - \chi_{\circlearrowright}\right) & \chi_{\circlearrowright} + \chi_{\circlearrowleft} \end{pmatrix} \begin{pmatrix} E_x \\ E_y \end{pmatrix} \\
&= \frac{\varepsilon_0}{2} \begin{pmatrix} \chi_{xx} & -i\chi_{xy} \\ i\chi_{xy} & \chi_{yy} \end{pmatrix} \begin{pmatrix} E_x \\ E_y \end{pmatrix}
\end{aligned} \tag{S.21}$$

where the off-diagonal susceptibility can be written

$$\chi_{xy} \approx \frac{i\rho \left|\mu_{fg}\right|^2}{(i\delta+\gamma)\,\varepsilon_0\hbar} \frac{\left(\gamma^2+\Delta^2\right)\left(\Omega_{\circlearrowright}^2-\Omega_{\circlearrowleft}^2\right)}{\left(\gamma^2+\Delta^2\right)\left(\Omega_{\circlearrowright}^2+\Omega_{\circlearrowleft}^2\right)+4\Omega_{\circlearrowright}^2\Omega_{\circlearrowleft}^2}, \tag{S.22}$$

which shows the nonreciprocity for $\chi_{xy} \neq 0$. When $\Omega \gg E$ is not well satisfied, the solution is solved entirely using numerical methods based on the full master equation. In addition, we have to consider the influence of atoms in and out of the interacting region due to the atomic motion or collision in the actual system, which leads to the incoherent transition between ground states. Therefore, the master equation needs to be rewritten as $d\rho/dt = -i[H,\rho] + \sum_{m,n=\pm M} \left\{\gamma\mathscr{L}\left(\sigma_{ge}^{mn}\right) + \gamma\mathscr{L}\left(\sigma_{gf}^{mn}\right) + J\mathscr{L}\left(\sigma_{gg}^{mn}\right)\right\}$, where $J$ is the relaxation coefficient of the incoherent transition. The relaxation effect reduces the atomic polarization, and the corresponding nonreciprocity is also affected, which is also confirmed by our numerical simulation results.

## II. RESULTS FOR TRANSVERSE-MAGNETIC (TM) MODES

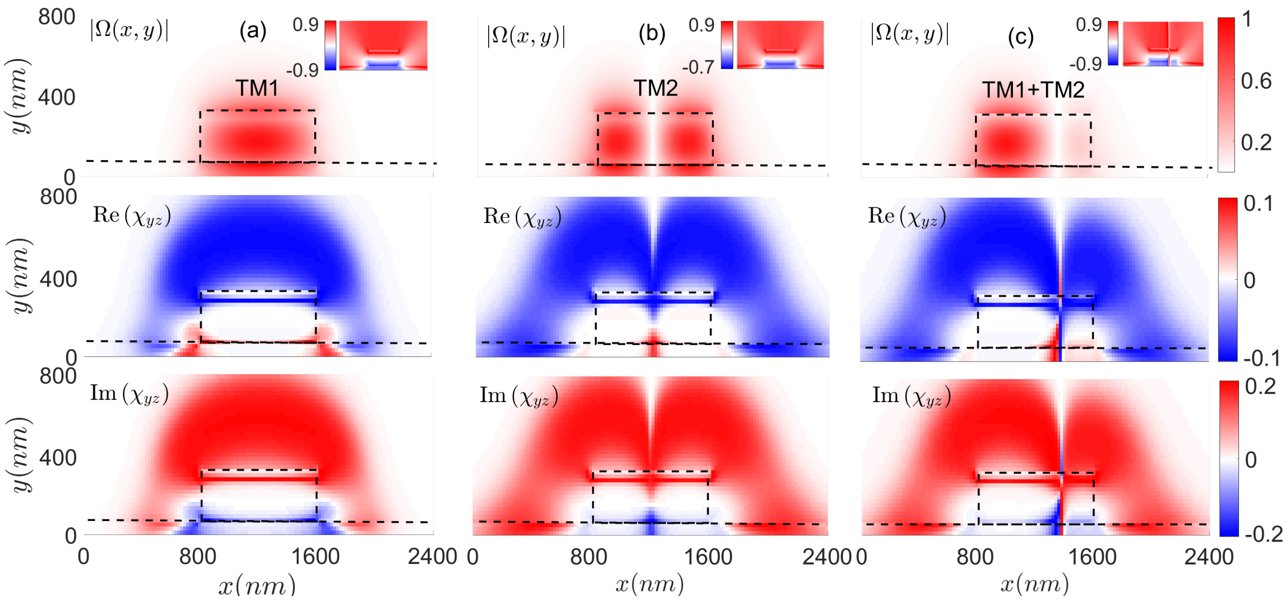


FIG. S2. The spatial distribution of the normalized light $|\Omega(x,y)|$ (top), the dispersion $\mathrm{Re}\,(\chi)$ (middle), and the absorption $\mathrm{Im}\,(\chi)$ (bottom) of the signal field with the detuning $\delta \simeq 0.5\gamma$ for the fundamental mode:TM1 (a), the second-order mode:TM2(b), and the superposition of both fundamental mode and second-order mode (c) for the TM modes. The black dotted line is the waveguide area and the small figure in the upper right corner represents the chirality $(\Omega_{\circlearrowright}-\Omega_{\circlearrowleft})/(\Omega_{\circlearrowright}+\Omega_{\circlearrowleft})$. The experimental realizable parameters are $\gamma = 10$ MHz, $\rho_a = 1.26\times10^{19}/\mathrm{m}^3$, $\mu_{fg} = 1.4\times10^{-29}$C.m, $\hbar = 1.055\times10^{-34}$J.s, $\varepsilon_0 = 8.85\times10^{-12}$F/m, $J = 10^{-4}\gamma$ and $\Omega = 10^2 E \simeq \gamma$

For the TM mode, we redefine $\circlearrowright = \overrightarrow{e_y} + i\overrightarrow{e_z}$ and $\circlearrowleft = \overrightarrow{e_y} - i\overrightarrow{e_z}$, and the corresponding distribution of cross section for the fundamental mode is shown in Fig. S2(a). The top panel is the normalized distribution of the fundamental mode, which is proportional to the control strength $|\Omega_{x,y}|$, and the inset in the upper right corner represents the chirality $(\Omega_{\circlearrowright}-\Omega_{\circlearrowleft})/(\Omega_{\circlearrowright}+\Omega_{\circlearrowleft})$ We find that the chiral field is mainly distributed on the top boundary of the waveguide, which is different from the TE mode. The middle and bottom panels in Fig. S2(a) are the real part $\mathrm{Re}\,(\chi_{yz})$ and the imaginary part $\mathrm{Im}\,(\chi_{yz})$ of the susceptibility, which show similar feature tothe chirality distribution. Since the imaginary part $\mathrm{Im}\,(\chi_{yz})$ of the susceptibility corresponds to absorption, this mode is very suitable for the nonreciprocal transmission of the light in the waveguide if the atoms are distributed on the top surface of the waveguide. The waveguide also supports the TM high-order modes and their superposition mode, as shown in Fig. S2(b) and (c), respectively. The spatial distribution shows different features with the TE modes.

The analytical and numerical results show that the distribution of the susceptibility is determined by the control field due to $|\overrightarrow{E}| \ll |\overrightarrow{\Omega}|$. When the weak signal approximation does not hold, the programmable susceptibility can show more complex spatial distribution. The mode of the signal field can be different from that of the control field. Except the control field, the probe mode can be also written as $E_{\circlearrowright(\circlearrowleft)}(x,y) = \xi E^1_{\circlearrowright(\circlearrowleft)}(x,y) + \sqrt{1-(\xi)^2}E^2_{\circlearrowright(\circlearrowleft)}(x,y)$, where $0 \le \xi \le 1$. At this point, the susceptibility is very sensitive to some parameters, such as the control detuning $\Delta$, the signal detuning $\delta$, and the intensities of the control $\Omega$ and the signal $E$. In addition, by employing the assisted level $|s\rangle$, we can design much more complex susceptibility distribution as required in principle. Based on the results above, we conclude that we can realize the SPMs by employing the high-order modes of the waveguide and other adjustable parameters.

## III. THREE-DIMENSIONAL PROGRAMMABILITY

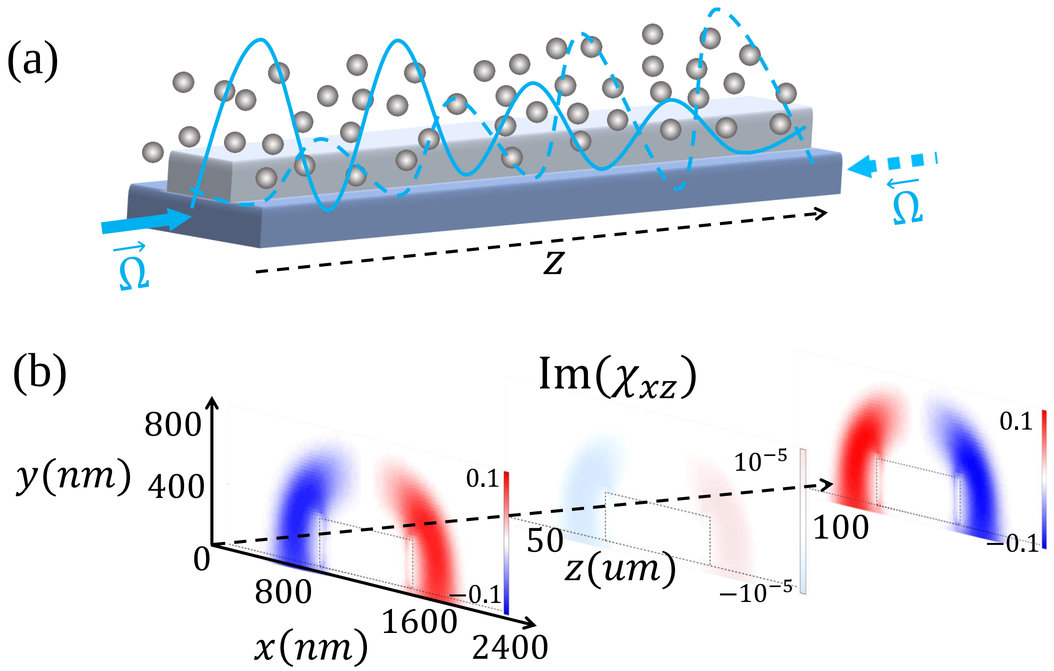


FIG. S3. (a) Schematic diagram of three-dimensional programmability by injecting two-way control lights. (b) Sectional views of the absorption distribution along the $z$ direction with the same strength of the two-way control lights, which can be modulated by changing the ratio between the two-way control lights.

The susceptibility for the signal field is determined by the control light due to $\Omega \gg E$, and the distribution of the control light keeps unchanged due to almost no absorption when the one-way control light travels along the $z$ direction, which means that the programmability is limited to two dimensions. Therefore, two-way control lights, which are injected into the waveguide from the two opposite directions, can be used to expand the programmability in the $z$ direction, where the control light gradually becomes weaker along the traveling direction $z$ due to the existence of the another control light from the opposite direction. The schematic diagram with two-way control lights is shown in Fig. S3 (a), where we label the control lights from the left and right directions as $\overrightarrow{\Omega}$ and $\overleftarrow{\Omega}$, respectively. The corresponding decomposition for the control lights can be written as $\Omega_{\circlearrowright(\circlearrowleft)} = \overrightarrow{\Omega}_{\circlearrowright(\circlearrowleft)} + \overleftarrow{\Omega}_{\circlearrowright(\circlearrowleft)}$, and we can calculate the susceptibility by the chiral light, which includes the control lights from both the left and right lights.

We know that the chiral distribution of the control light for the certain waveguide mode keeps unchanged, but the chirality is reversed for two-way control lights. It is natural that the ratio between the control lights traveling in opposite directions changes along the $z$ direction due to the absorption, and the corresponding traveling equations can be written as

$$\frac{\partial \overrightarrow{\Omega}(z)}{\partial z} = ik\frac{\mathbf{P}(z)}{\varepsilon_0}, \tag{S.23}$$

$$\frac{\partial \overleftarrow{\Omega}(l-z)}{\partial z} = ik\frac{\mathbf{P}(l-z)}{\varepsilon_0}, \tag{S.24}$$

where the positions in the $z$ direction for the right and left traveling control lights are labeled as $z$ and $l-z$, respectively. We can obtain the stable solutions through repeated iterations, and the corresponding susceptibility is shown in Fig. S3 (a), where we assume the same input initial strengths $\overrightarrow{\Omega}(0) = \overleftarrow{\Omega}(l)$. In addition to the two-dimensional distribution of the susceptibility, the numerical results show that the susceptibility changes along the $z$ direction, and there is little absorption at the middle of the waveguide $z = l/2$, where the control lights are very weak. We also observe the anti-symmetry susceptibility at both ends of the waveguide, which is attributed to the reversed chirality for the opposite control lights injected into the waveguide. If we change the ratio of the two-way control lights, we can further tune the susceptibility in the $z$ direction, which means that the programmability can be expanded into the three-dimensional space in principle.

## IV. DYNAMICAL EVOLUTION

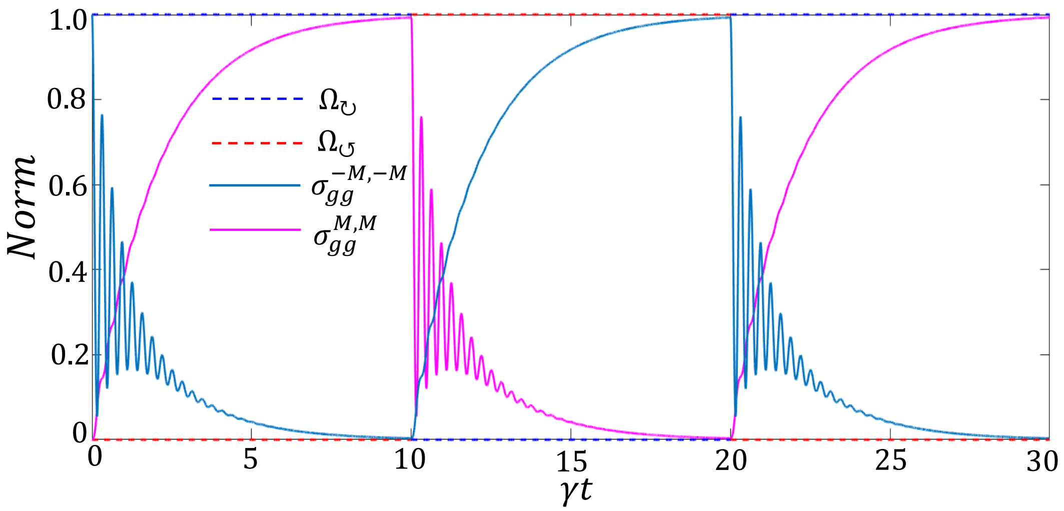


FIG. S4. The dynamical evolution (solid lines) of the atomic population when quickly switching the control light (dotted lines), where we have normalized the control light (Norm). The oscillation phenomenon gradually disappears and the system tends to stabilize when the dimensionless parameter $\gamma t \approx 10$. Here we assumed that the strength of the control lights ($\Omega_{\circlearrowright}$ and $\Omega_{\circlearrowleft}$) is same, so the periodic oscillations of the atomic population are translationally symmetric.

The previous results are based on the steady conditions. However, we also concern the dynamical process to study the switching speed and the signal distortion of the nonreciprocal process, which can be further extended to the programmability in time. From the master equation, we obtain the dynamical evolution of the atomic transition

$$\frac{d}{dt}\sigma_{\mathrm{eg}}^{M,-M} = -i\Delta\sigma_{\mathrm{eg}}^{M,-M} - i\Omega_{\circlearrowright}\left(\sigma_{\mathrm{ee}}^{M,M} - \sigma_{\mathrm{gg}}^{-M,-M}\right) - \gamma\sigma_{\mathrm{eg}}^{M,-M}, \tag{S.25}$$

$$\frac{d}{dt}\sigma_{\mathrm{eg}}^{-M,M} = -i\Delta\sigma_{\mathrm{eg}}^{-M,M} - i\Omega_{\circlearrowleft}\left(\sigma_{\mathrm{ee}}^{-M,-M} - \sigma_{\mathrm{gg}}^{M,M}\right) - \gamma\sigma_{\mathrm{eg}}^{-M,M}. \tag{S.26}$$

We know that the atomic population is determined by the control light $\Omega$, which reflects the susceptibility of the unsteady process. In Fig. S4, we study the dynamical process when the control light is quickly switched, as labelled by the dotted lines, which has been normalized. We numerically calculate the corresponding atomic population (solid lines) as the function of the time $t$, and it is noticed that there are periodic oscillations of the atomic population, which means that the atoms are an unstable state. We observe that the time reaching the steady state for the atom is inversely proportional to the atomic decay rate, that is $\tau \propto 1/\gamma$, which is consistent with evolution equations. Here we assume the decay rate $\gamma = 10$ MHz, and the corresponding duration is $\tau \approx 0.1$ us. It has been calculated that the susceptibility is determined by the atomic population of ground states. Therefore, the switch functionality of susceptibility tensor has a high speed, which depends on the atomic decay rate $\gamma$.

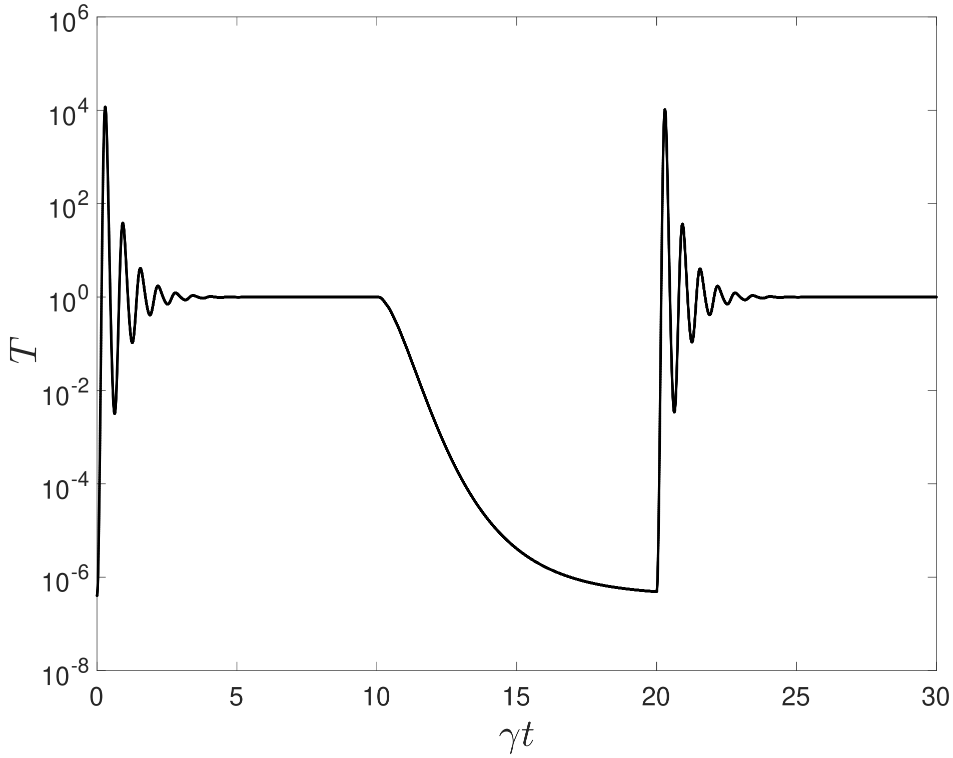


FIG. S5. The dynamical transmission of the signal field when the control light is quickly switched. At the beginning, the control light and the signal light are in the same direction, and the signal light has little absorption. On the contrary, an interesting temporal amplification effect $T > 1$ of the signal field is observed, which is attributed to population inversion in the unstable process. We also notice that the oscillation period is not consistent with the population of the ground states, because the strength of the signal is also related to the population of the excited state in the unsteady state. When the transmission direction of the signal light is in the opposite with the control light, there is a huge absorption for the signal light, and the switching speed is proportional to the atomic decay rate $\gamma$.

Considering the slowly varying envelop approximation, the dynamic evolution of the optical field can be given by the equation [1]

$$\frac{1}{c}\frac{\partial \mathbf{E}}{\partial t}+\frac{\partial \mathbf{E}}{\partial z}=ik\frac{\mathbf{P}}{\varepsilon_0}, \tag{S.27}$$

where $c$ is the vacuum speed of light, $k=|\mathbf{k}|$ is the wave vector of the signal field, and the the polarization $\mathbf{P}$ is the electric dipole moment per unit volume, which can be written as $\mathbf{P}=\varepsilon_0\overleftrightarrow{\chi}\cdot\mathbf{E}$ [3, 4], where $\varepsilon_0$ is the vacuum permittivity and $\overleftrightarrow{\chi}$ is the susceptibility tensor. Although we need to consider the unsteady susceptibility $\mathbf{P}=\mathbf{P}(t)$, the dynamical evolution of the optical field can be simplified as

$$\frac{\partial \mathbf{E}(t)}{\partial z}\approx ik\frac{\mathbf{P}(t)}{\varepsilon_0}, \tag{S.28}$$

where we have ignored the transmission time of the light along the waveguide with the length $L$ due to $L/c \ll 1/\gamma$. It means that the transmission has a similar dynamical characteristic with the susceptibility, which is confirmed by the Fig. S5, and the transmission is defined as $T=|E(t,z=L)/E(t,z=0)|^2$. We observe that it takes the same duration for the transmission to reach the steady state as the susceptibility, and therefore the establishment of non-reciprocity is also proportional to $1/\gamma$. We can realize the high-speed switching functionality of our susceptibility-programmable medium, and the speed of nonreciprocal switch is limited by the atomic decay rate $\gamma$. In principle, the switching speed can be further improved by raising the temperature or injecting an inert gas into the atomic cell to increase the atomic decay rate $\gamma$. In addition, we also observe an interesting temporal amplification effect of the signal field, which is attributed to population inversion in the unstable process.

The inconsistency of oscillation period further confirms that the signal transmission also depends on the population of excited states in the unstable state. Such behavior reveals rich physics behind the susceptibility-programmable medium studied in this work, which appeals further exploration of the programmable function, such as time programmability and dynamical nonreciprocal amplification in future works.

## V. SIGNAL DISTORTION

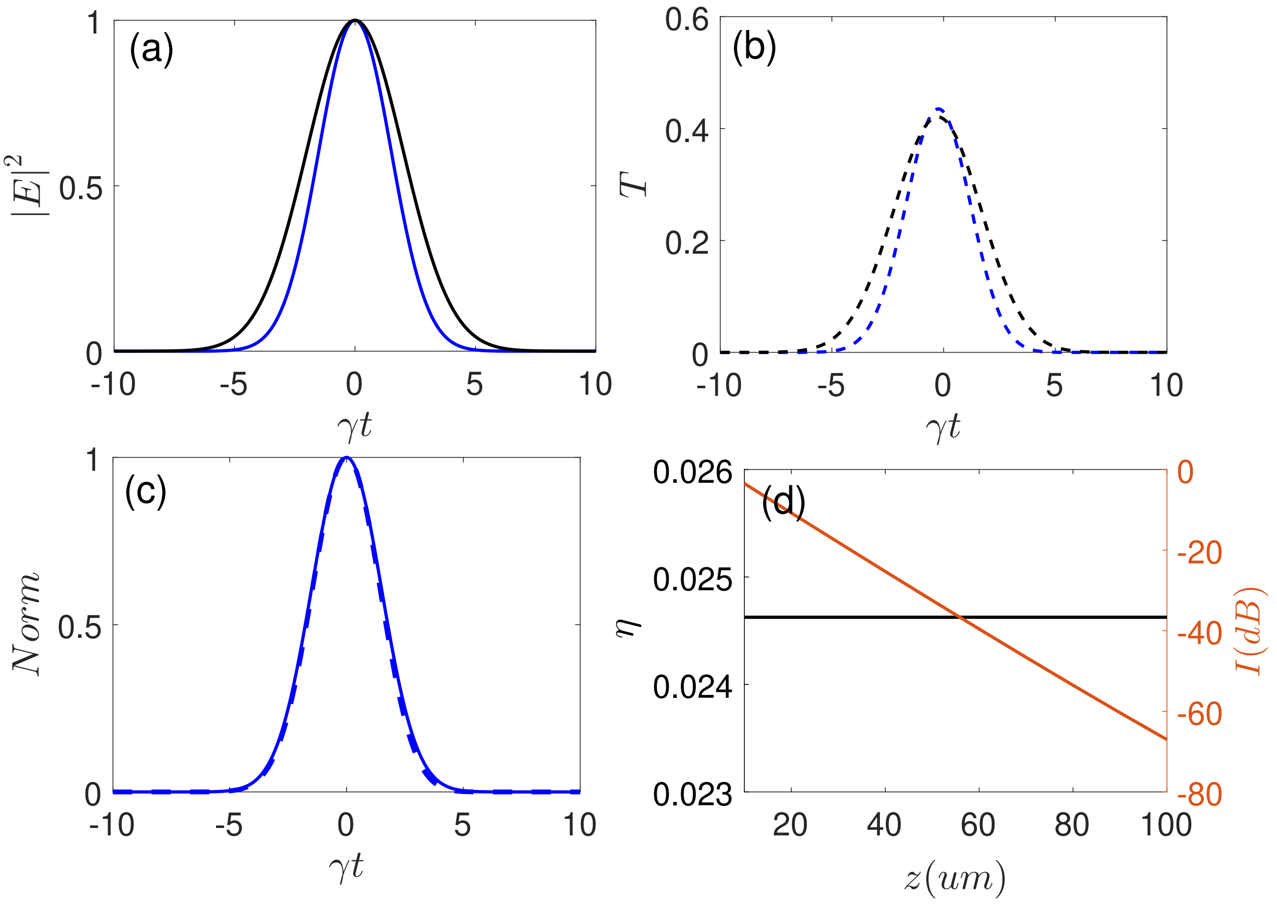


FIG. S6. Distortion for a pulse signal after transmitting along the waveguide. (a) The pulse signals $E(t) \propto \exp\left(-t^2/|\Delta t|^2\right)$ for $\Delta t = 4/\gamma$ (the black line) and $\Delta t = 3/\gamma$ (the blue line). (b) The pulse waveform of the signal that should have passed through the waveguide, where $T < 1$ means that there is a little absorption. (c) Comparison of pulse waveforms after the normalization, which shows a slight distortion even $\Delta t = 3/\gamma$. (d) The degrees of distortion and isolation vary with the length of the waveguide $z$, and the numerical results show that the distortion degree changes little with the increase of the length of the waveguide after normalization. Other parameters are same with the parameters in FIG. 3.

In addition to isolation of nonreciprocal transmission and the switching speed for the signal transmission, we need to consider the distortion when the pulse signal comes through the waveguide. Here we assume that the signal is $E(t) \propto \exp\left(-t^2/|\Delta t|^2\right)$, which changes with the time, as shown in Fig. S6 (a). The black and blue lines are corresponding to the different pulses $\Delta t = 4/\gamma$ and $\Delta t = 3/\gamma$, respectively. When the pulse signal and the control light are transmitted in the same direction in the waveguide, we observe a certain loss of the signal light that passes through the waveguide, which is plotted in Fig. S6 (b). However, the profile of the pulse signal keeps almost unchanged and we plot the normalization of the transmitting signal (the dotted line) in Fig. S6 (c), where the waveforms of the input and output signal light almost coincide.

It is obvious that the distortion degree is related to the pulse width $\Delta t$, which is attributed to that the dispersion is zero when $\omega = 0$, and the frequency width is smaller by the Fourier transform from the time space to the frequency space for longer pulse. Here we define the distortion degree $\eta = \int |Norm(t) - E(t)|^2 dt / \int |E(t)|^2 dt$. It is calculated that the distortion degree becomes smaller with the increasing of the pulse width, and meanwhile the isolation is improved in FIG. 4(b). The numerical results show that the distortion keeps almost unchanged with the transmitting length $z$ for the certain pulse width, and the isolation can always be improved, which is plotted in Fig. S6 (d).

## VI. EXPANDED APPLICATIONS

Based on the concept of susceptibility-programmable medium, there are many important applications in addition to the non-reciprocal transmission. The core concept of controlling the susceptibility tensor with high spatial and temporal resolution is a fundamental breakthrough that can be extended to various other photonic structures, such as metasurfaces, photonic crystals, and optical fibers. The waveguide example serves as a proof-of-concept demonstration that highlights the capabilities and practical relevance of the proposed approach. Next, we provide some other concrete applications: the mode conversion, the tunable optical interference, and the chirality detection.

### A. Mode conversion

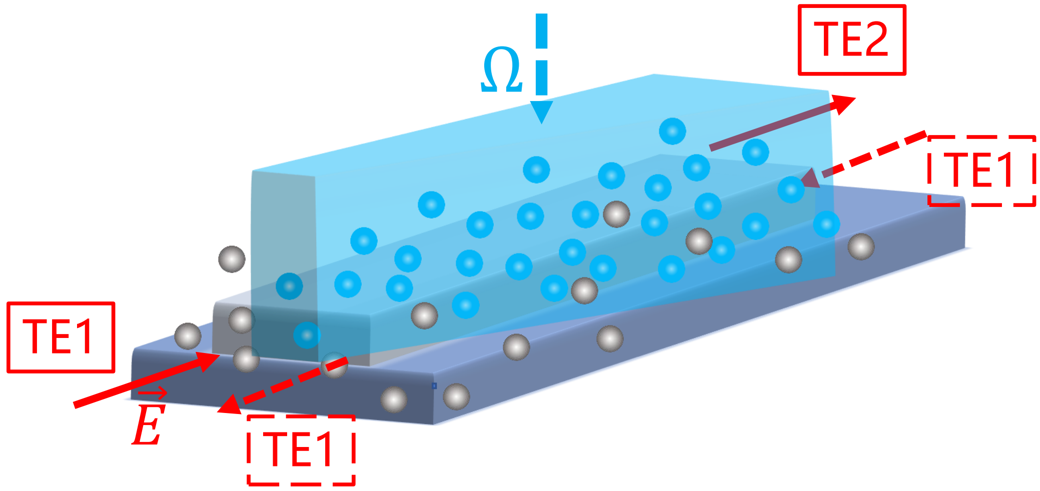


FIG. S7. Schematic diagram of mode conversion. We employ the control light with a certain spatial shape through the free space onto the waveguide surface, which is corresponding to the blue area. Due to the polarization characteristics of the control light, the atoms in the blue area are excited, which affect the transmission of the signal field. For the high-density atoms, the changes in refractive index around the waveguide affect the waveguide mode, and we can realize the nonreciprocal mode conversion that depends on the transmission direction if we combine the chirality of the waveguide.

As shown in Fig. S7, we plot the schematic diagram of mode conversion. We have known that there is a significant change of up to 0.1 in the effective refractive index for the atomic density $\rho_a = 1.26 \times 10^{19}/\mathrm{m}^3$. Therefore, the changes in refractive index around the waveguide will change the waveguide mode for the high-density atoms, and we can achieve the mode conversion when the signal transmits in the waveguide by designing the spatial configuration of the control light, labelled by the blue area. When the chirality of the control light and the chirality of the signal light are the same, the transmission mode of the signal remains unchanged (dotted lines). On the contrary, the mode of the signal field can change from TE1 to TE2 during the transmission of signal light (solid lines). To reduce the effect outside the blue area, we pump the atoms into the assisted state $|s\rangle$. In conclusion, we can realize the nonreciprocal mode conversion by employing both the spatial configuration and chirality of the control light.

### B. Tunable optical interference

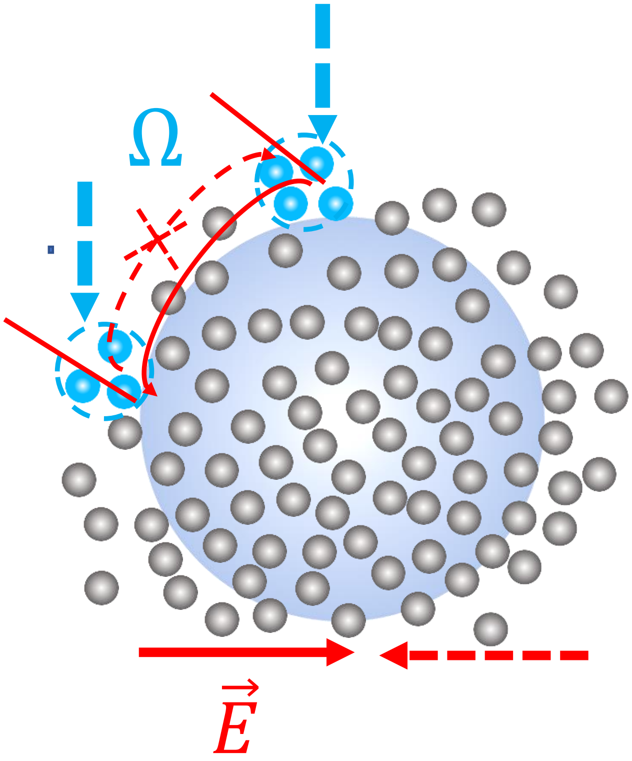


FIG. S8. Schematic diagram of tunable optical interference in space and time. In principle, the high-density atoms can be seen as scattered particles for a microsphere cavity by the control light with the special spatial configuration. The optical interference can be realized by two or more scattered particles, which can be moved and switched off.

We know that the state $|s\rangle$ is an idle energy level, whose transition to other energy levels are far off-resonance with the control and probe fields. Thus, the interaction between the atom and both the control and signal fields are switched off when the atom is prepared to the state $|s\rangle$, and then atom is transparent to the signal. In order to further utilize the advantages of assisted state, we design a tunable optical interference, as shown in Fig. S8, where the gray atoms are pumped into the state $|s\rangle$. For the control light in free space, its spatial distribution and switch are relatively easy to adjust, and therefore we can realize the tunable optical interference in space and time. The interference intensity can be changed by the size and position of scattered particles, which depends on the control light.

In addition, we also notice that the chirality of the traveling wave mode in the microsphere cavity also relies on the transmitting direction, as shown by the red lines in Fig. S8. When the chirality of the signal light and the control light around the microcavity is opposite, the interference phenomenon of the signal light will occur due to the scattering particles composed of atoms. Due to the chirality of the signal field on the surface of the microcavity being related to the direction of incidence, this interference phenomenon is also nonreciprocal. In summary, we can achieve adjustable nonreciprocal interference on this device.

### C. Polarization and chirality detection

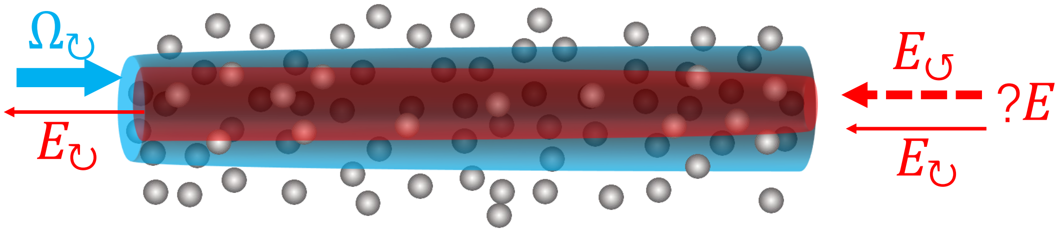


FIG. S9. Schematic diagram of mode conversion

In classical and quantum information processing, the detection and analysis of signal polarization is crucial, and its accuracy is limited by the purification of different polarized light. In Fig. S9, we propose a polarization detection scheme for signal light by utilizing the advantage of easy adjustment of the light field in free space. Under the condition of determining the control of optical polarization, we can achieve chiral detection of an unknown signal. The part of the signal light that is opposite to the polarization of the control light is absorbed, and the same part is transmitted. The polarization of signal light can be determined through the detection of signal transmittance. Obviously, its detection accuracy is limited by the polarization of the control light, which can be improved by cascading multiple such devices. In the previous discussion on the waveguide, its chiral distribution characteristics depend on the size, structure, and material of the waveguide. Under the conditions of determining atomic density and excitation mode, the isolation degree is limited by the configuration of the waveguide. Therefore, we can analyze the chiral characteristics of devices with different complex configurations by measuring the isolation of transmission.

In addition, the atomic grating can be also constructed by injecting two-way pump idle lights, and this type of grating is not only dynamically adjustable, but also has chiral properties. In conclusion, we can combine the spatial programmability with the temporal programmability, and the hybrid programmability can be realized by multi-dimensional regulation. The ability to control the optical susceptibility with high spatial resolution and tunability could lead to significant advancements in various research fields, including optical signal processing, imaging, sensing, and quantum information processing.

---

* These two authors contributed equally to this work.
† clzou321@ustc.edu.cn
‡ xbz@ustc.edu.cn
[1] M. O. Scully and M. S. Zubairy, "Quantum optics," (1999).
[2] R. W. Boyd, *Nonlinear optics* (Academic press, 2020).
[3] A. Momeni, H. Rajabalipanah, A. Abdolali, and K. Achouri, "Generalized optical signal processing based on multioperator metasurfaces synthesized by susceptibility tensors," Physical Review Applied **11**, 064042 (2019).
[4] M. Kauranen, J. J. Maki, T. Verbiest, S. Van Elshocht, and A. Persoons, "Quantitative determination of electric and magnetic second-order susceptibility tensors of chiral surfaces," Physical Review B **55**, R1985 (1997).
